# Supplementary material for: NapierOne: A modern mixed file data set alternative to Govdocs1
Source: arXiv:2201.08154 source file (2022-01-20)
Supplement: Supplementary file 1 [file appendix.tex]

\section{Decrypted file modification}\label{introduction}
commands used to recreate header and footer information in decrypted files
\begin{verbatim}
NotPetya
header reconstruction for pdf
printf "\x25\x50\x44\x46\x2d\x31\x2e\x35\x0a\x25\xc7\xec\x8f\xa2\x0a\x35" | cat - pdf-decrypted.pdf > reconstructed-pdf.pdf

header reconstruction for xlsx
printf "\x50\x4b\x03\x04\x14\x00\x06\x00\x08\x00\x00\x00\x21\x00\x7c\x6c" | cat - excel-decrypted.xlsx > reconstructed-xlsx.xlsx
we then need to cut off the last 3 bytes
dd if=reconstructed-xlsx.xlsx of=reconstructed-xlsx1.xlsx bs=$((`cat reconstructed-xlsx.xlsx| wc -c` - 3)) count=1

header reconstruction for doc
printf "\xd0\xcf\x11\xe0\xa1\xb1\x1a\xe1\x00\x00\x00\x00\x00\x00\x00\x00" | cat - Word-decrypted.doc > reconstructed-doc.doc

header reconstruction for dox
printf "\x50\x4b\x03\x04\x14\x00\x06\x00\x08\x00\x00\x00\x21\x00\x09\x24" | cat - Word-decrypted.docx > reconstructed-docx.docx
we then need to cut off the last 7 bytes
dd if=reconstructed-docx.docx of=reconstructed-docx1.docx bs=$((`cat reconstructed-docx.docx| wc -c` - 7)) count=1
    
\end{verbatim}
